# Supplementary material for: Colour symmetry and altermagnetic-like spin textures in noncollinear antiferromagnets
Source: arXiv:2501.02947 ancillary file (2025-06-20)
Supplement: Supplementary file 1 [file Colour_symmetry-v5_Supplementary.pdf]

# Supplemental Information: Colour symmetry and altermagnetic-like spin textures in collinear altermagnets

Paolo G. Radaelli
*Clarendon Laboratory, Department of Physics, University of Oxford, Oxford, OX1 3PU, United Kingdom*[*]

Gautam Gurung
*Trinity College, University of Oxford, Oxford, OX1 3BH, United Kingdom*[†]

## I. COLOUR GROUPS AS PROPER SUPERGROUPS OF SPIN GROUPS

In this section, we provide an example of a magnetic structure described by a colour group that is a proper supergroup of the corresponding spin group. Fig. S1 display the proposed magnetic structure of the high-filed phase of TmAgGe.[1] This phase is non-collinear with a strongly ferromagnetic component *not* due to SOC. The paramagnetic parent phase has symmetry $P\bar{6}2m$, with the magnetic Tm atoms being on symmetry-equivalent sites. Upon magnetic ordering, the magnetic sites split into two orbits: the sites marked as G and B remain symmetry equivalent (by 2-fold rotation), while the R site is no longer equivalent and is allowed to have a different magnetic moment (it is the only site aligned with the magnetisation). The MSG/MPG of the ordered structure are $Am'm'2$ and $m'm'2$, the 2-fold axis being aligned with the magnetisation. Since the 'fan' of magnetic moments cannot be generated by a single crystallographic point group, the two sites must also be treated separately within the SG framework. One can employ for both sites the SG $m_2m_12_2$ with the 2-fold axis acting in spin space being parallel to the magnetisation. However, within the CG framework, the three sites can remain equivalent, at least at the level of approximate symmetry. The appropriate CG is $\{\bar{6}2m|mm2|m\}$, which has 12 symmetry elements compared to the 4 symmetry elements of the SG and MPG. A tensorial expansion of the spin texture can be easily constructed within this framework, and it is expected to have higher symmetry than to the equivalent MPG/SG constructions. Note that the group $H' = mm2$ that leaves one colour invariant is a *proper* subgroup of $\bar{6}2m$ (this is always the case for non-trivial CGs), and is also isomorphic to the SG $m_2m_12_2$.

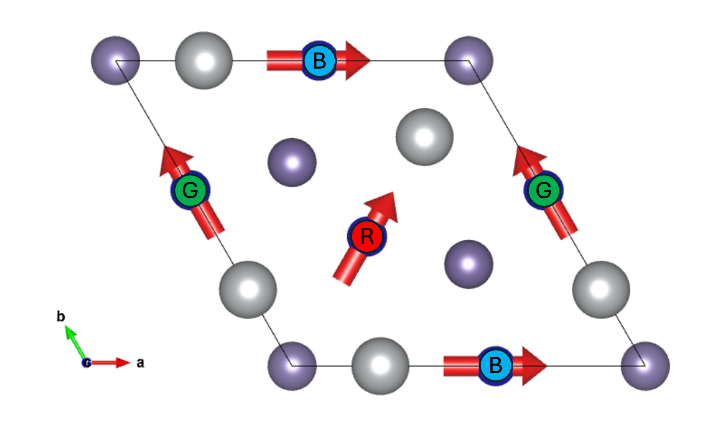


FIG. S1. *ab*-plane projection of the proposed magnetic structure of TmAgGe above the metamagnetic transition. Magnetic Tm sites are shown with an arrow. Large and small balls represent Ag and Ge, respectively.[1]

## II. SPIN-RESOLVED BAND STRUCTURE OF $Mn_3GaN$

Fig. S2 and S3 display the spin-resolved band structure with/without spin orbit coupling in the lower/upper row for $Mn_3$ GaN in the $\Gamma^{5g}$ and $\Gamma^{4g}$ phases along high symmetry paths in the first Brillouin zone (see Fig. S4). Color shows the strength of the spin components $\langle s_x\rangle$, $\langle s_y\rangle$, and $\langle s_z\rangle$. The colorbar scale is from -0.5 to 0.5 for $\langle s_x\rangle$ and $\langle s_y\rangle$ components. The scale is reduced by a factor of 10 for the smaller $\langle s_z\rangle$ components. The $x, y$, and $z$ direction is along $[1\bar{1}0]$, $[11\bar{2}]$, and $[111]$ direction. The inset shows the spin splitting of fermi bands along the $\Gamma$ to $R$ in presence of spin orbit coupling in $\Gamma^{4g}$ phase. This DFT calculated results agree with the prediction of CPG analysis.

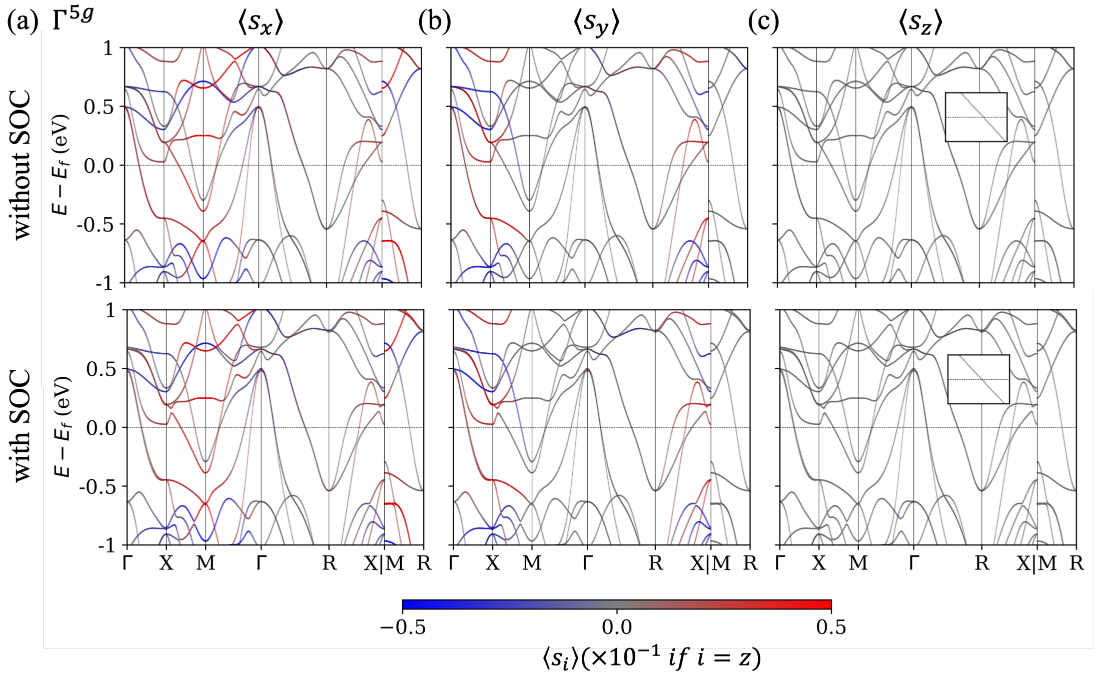


FIG. S2. (Colour online) Spin projected band structure (a) $\langle s_x \rangle$, (b) $\langle s_y \rangle$, and (c) $\langle s_z \rangle$ with/without spin orbit coupling (SOC) in lower/upper row for $Mn_3GaN$ in noncollinear antiferromagnetic $\Gamma^{5g}$ phase along high symmetry paths in the simple cubic first Brillouin zone. The $x, y$, and $z$ direction is along $[1\bar{1}0], [11\bar{2}]$, and $[111]$ direction. The inset shows the *absence* of spin splitting of fermi bands along the $\Gamma$ to $R$ in presence of spin orbit coupling.

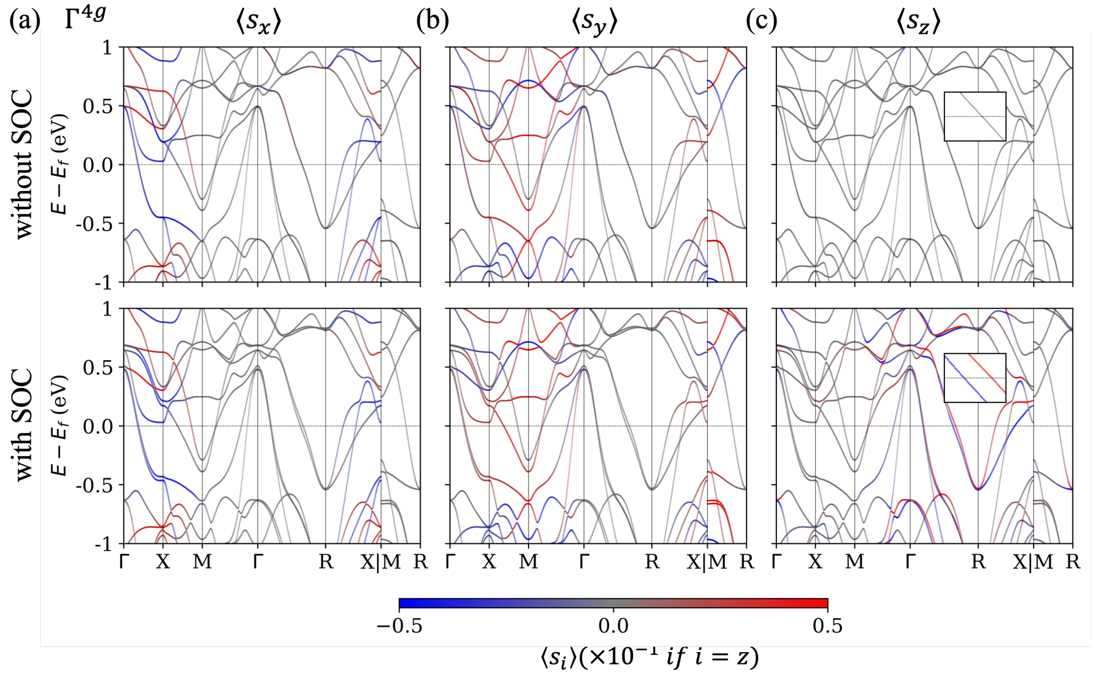


FIG. S3. (Colour online) Spin projected band structure (a) $\langle s_x \rangle$, (b) $\langle s_y \rangle$, and (c) $\langle s_z \rangle$ with/without spin orbit coupling (SOC) in lower/upper row for $Mn_3GaN$ in noncollinear antiferromagnetic $\Gamma^{4g}$ phase along high symmetry paths in the simple cubic first Brillouin zone. The $x, y$, and $z$ direction is along $[1\bar{1}0], [11\bar{2}]$, and $[111]$ direction. The inset shows the *presence* of spin splitting of fermi bands along the $\Gamma$ to $R$ in presence of spin orbit coupling.

## III. FERMI SURFACE OF $Mn_3GaN$

Fig. S4 displays the fermi surface of $\Gamma^{4g}$ phase of $Mn_3GaN$ in presence of spin orbit coupling (SOC). The 3D view shows that there are five Fermi surfaces, labeled from 0 to 4 as we move from $\Gamma$ to the $R$ high-symmetry points. Band 0 (blue) is overlapped by Band 1 (cyan). The projection plane (gray shaded region) contains the $\Gamma$ point and is normal to the (1,1,1) direction. This plane does not contain band 4(red). In the presence of spin-orbit coupling (SOC), there is a band splitting between band 3 and band 4 (see Fig. S3).

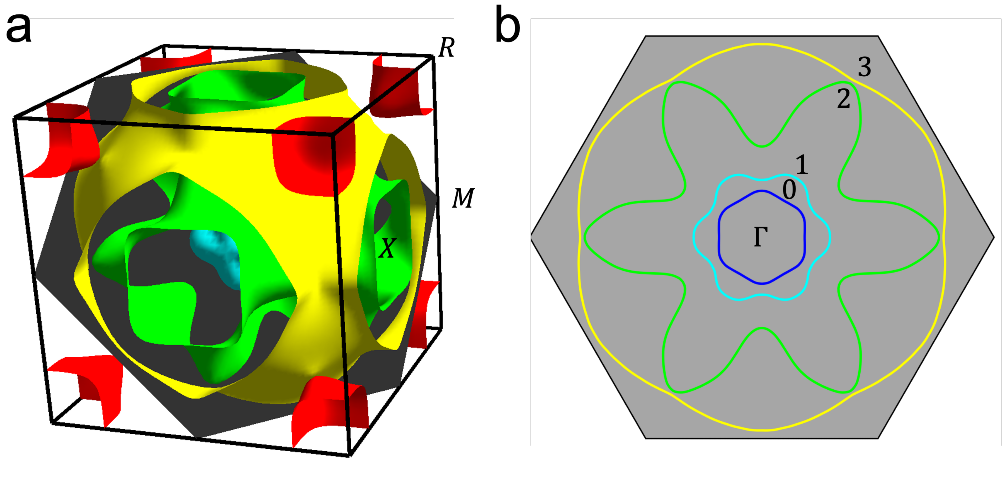


FIG. S4. (Colour online) Fermi surface of $Mn_3GaN$.(a) 3D view of the Fermi surface with labelled high symmetry points. The grey shaded region represents the plane cut perpendicularly to the (1,1,1) direction including the $\Gamma$ point. (b) 2D planar projection on the plane cut shown with an outline of the BZ, calculated using DFT for the $\Gamma^{4g}$ phase with SOC. The bands are labeled from $0-3$ as we move radially outward from the $\Gamma$ point. Colors represent the band index 0 to 4 (blue, cyan, yellow, lime, and red).

## IV. DECOMPOSITION OF THE FERMI SURFACE SPIN TEXTURE ONTO TENSORIAL EXPANSIONS

The projected spin texture of the Fermi surface on the equatorial section as shown in Fig. S4 was decomposed onto the radial, tangential and axial components. Axial components are non-zero only in the presence of spin orbit coupling. CG tensor decompositions were performed up to tensorial rank 18, while MPG decompositions of the axial components were to rank 13. Only a small number of parameters are necessary to describe the tensorial expansions onto the high-symmetry equatorial section (the parametrised functional forms are reported in the first lines of Table S1/S2). These parameters were then fitted onto the spin textures calculated by DFT (see Table S1/S2) for the $\Gamma^{4g}/\Gamma^{5g}$ phase with or without SOC. The results of these fits are displayed graphically in Fig. S5-S7 and Fig. 7 of the main text, showing good agreement between the DFT calculated results with the predicted tensorial expansion.

TABLE S1. Fitting parameters for radial, tangential and axial components projected on the fermi surface of $Mn_3GaN$ in $\Gamma^{4g}$ phase. $[A_0, A_1, A_2, ..]/(A_0, A_1, A_2, ..)$ represents fitting parameter with/without spin orbit coupling respectively.

| $\Gamma^{4g}$ | Radial $\sum_{n=0}^{3} A_n \sin[3(2n+1)\phi]$ | Tangential $\sum_{n=0}^{3} A_n \cos[3(2n+1)\phi]$ | Axial $\sum_{n=0}^{2} A_n \cos[3(2n)\phi]$ |
|---|---|---|---|
| Band 0 | ( 0.161, -0.016, 0.003, -0.001) | ( 0.397, -0.058, 0.001, -0.002) | |
| | [ 0.159, -0.011, 0.002, -0.001] | [ 0.384, -0.043, 0.001, -0.002] | [ 0.0069, -0.0032, 0.0002] |
| Band 1 | ( 0.209, -0.001, -0.001, 0.001) | ( -0.202, 0.083, -0.012, 0.003) | |
| | [0.205, -0.001, 0.000, 0.001] | [-0.197, 0.072, -0.007, 0.002] | [0.0115, 0.0017, -0.0012] |
| Band 2 | ( -0.075, 0.069, 0.019, 0.016) | ( 0.162, -0.054, -0.031, -0.008) | |
| | [ -0.065, 0.066, 0.019, 0.017] | [ 0.168, -0.052, -0.029, -0.006] | [ -0.0121, 0.0032, 0.0036] |
| Band 3 | ( 0.225, -0.125, -0.065, -0.027) | ( 0.389, -0.100, -0.034, -0.030) | |
| | [ 0.208, -0.111, -0.071, -0.027] | [ 0.386, -0.104, -0.036, -0.032] | [ 0.0123, -0.0148, 0.0012] |

TABLE S2. Fitting parameters for radial, tangential and axial components projected on the fermi surface of $Mn_3GaN$ in $\Gamma^{5g}$ phase.$[A_0, A_1, A_2, ..]/(A_0, A_1, A_2, ..)$ represents fitting parameter with/without spin orbit coupling respectively. For the axial component, the coefficient $A_0$ is $= 0$ by symmetry.

| $\Gamma^{5g}$ | Radial $\sum_{n=0}^{3} A_n \cos[3(2n+1)\phi]$ | Tangential $\sum_{n=0}^{3} A_n \sin[3(2n+1)\phi]$ | Axial $\sum_{n=1}^{2} A_n \sin[3(2n)\phi]$ |
|---|---|---|---|
| Band 0 | ( 0.396, -0.058, 0.001, -0.002) | ( -0.161, 0.016, -0.003, 0.001) | |
| | [ 0.379, -0.042, 0.001, -0.002] | [ -0.155, 0.010, -0.002, 0.001] | [ 0.0009, -0.0000] |
| Band 1 | ( -0.201, 0.082, -0.012, 0.003) | ( -0.209, 0.002, 0.000, -0.001) | |
| | [ -0.196, 0.071, -0.007, 0.002] | [ -0.206, 0.002, -0.000, -0.001] | [ -0.0082, 0.0003] |
| Band 2 | ( 0.163, -0.054, -0.030, -0.008) | ( 0.074, -0.069, -0.019, -0.016) | |
| | [ 0.168, -0.053, -0.030, -0.007] | [ 0.065, -0.066, -0.019, -0.017] | [ 0.0123, 0.0050] |
| Band 3 | ( 0.388, -0.101, -0.035, -0.030) | ( -0.224, 0.125, 0.065, 0.028) | |
| | [ 0.386, -0.105, -0.033, -0.030] | [ -0.205, 0.113, 0.071, 0.027] | [ -0.0110, -0.0068] |

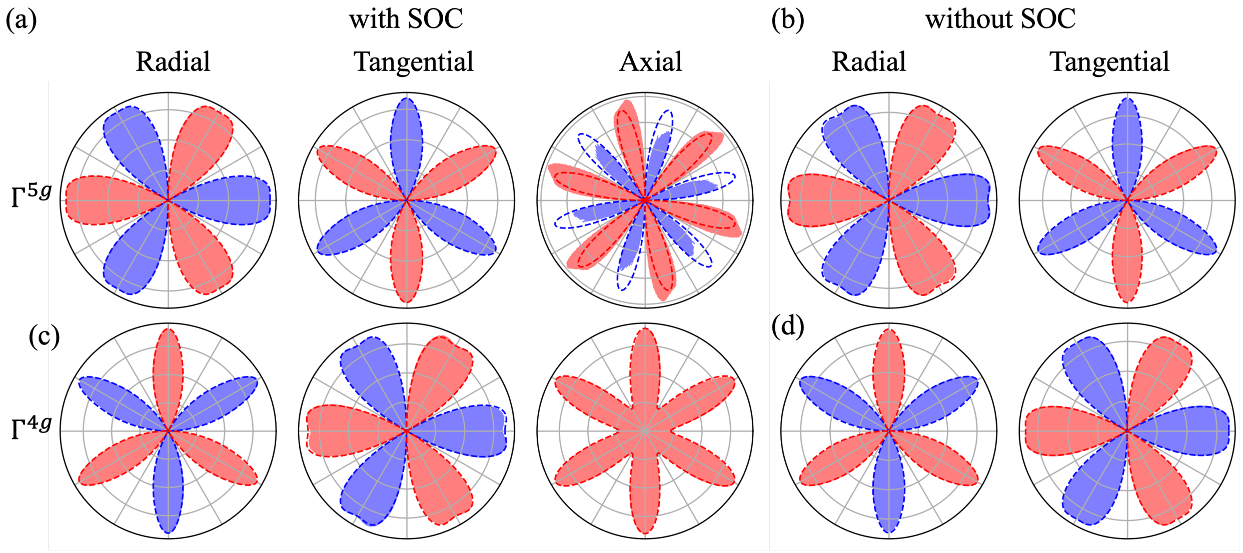


FIG. S5. (Colour online) Decomposition of the Band-0 spin textures calculated with DFT (solid blocks) and with the corresponding tensorial fits (dashed lines) for $\Gamma^{5g}$ (top row) and $\Gamma^{4g}$ (bottom row). Red/Blue indicate positive/negative components (note the $\mathbf{k}/-\mathbf{k}$ symmetry). Panels (a)/(c) and (b)/(d) were calculated, respectively with and without SOC (see text). The outer circles in the plots corresponds to amplitudes for the radial, tangential and axial components of [0.340,0.169,0.001]/[0.173,0.342,0.010] or (0.351,0.181)/(0.181,0.351) for the $\Gamma^{5g}/\Gamma^{4g}$ phase, respectively, with [] or without () SOC respectively.

* Corresponding author: p.g.radaelli@physics.ox.ac.uk
† Corresponding author: gautam.gurung@trinity.ox.ac.uk
1 S. Baran, D. Kaczorowski, A. Arulraj, B. Penc, and A. Szytuła, Journal of Magnetism and Magnetic Materials **321**, 3256 (2009).

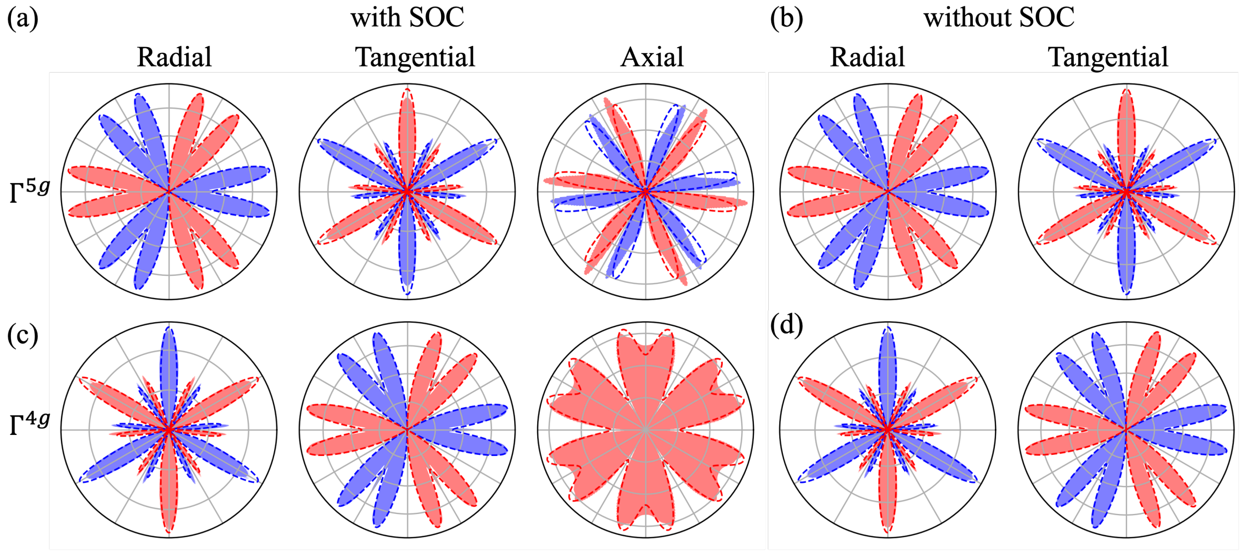


FIG. S6. (Colour online) Decomposition of the Band-2 spin textures calculated with DFT (solid blocks) and with the corresponding tensorial fits (dashed lines) for $\Gamma^{5g}$ (top row) and $\Gamma^{4g}$ (bottom row). Red/Blue indicate positive/negative components (note the $\mathbf{k}/-\mathbf{k}$ symmetry). Panels (a)/(c) and (b)/(d) were calculated, respectively with and without SOC (see text). The outer circles in the plots corresponds to amplitudes for the radial, tangential and axial components of [0.184,0.125,0.017]/[0.123,0.180,0.016] or (0.179,0.133)/(0.133,0.179) for the $\Gamma^{5g}/\Gamma^{4g}$ phase, respectively, with [] or without () SOC respectively.

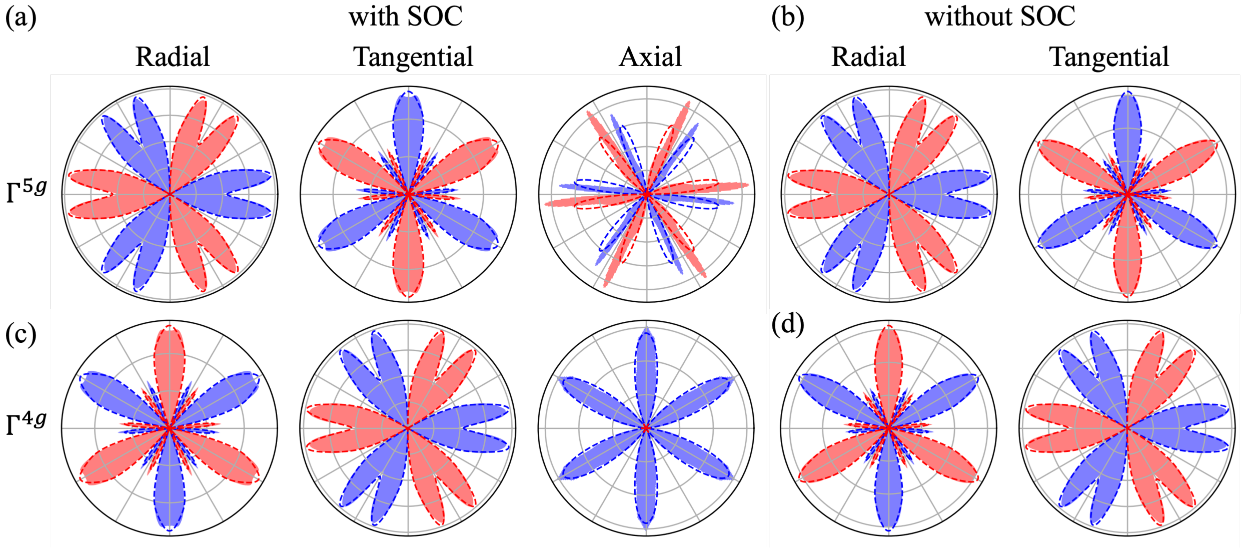


FIG. S7. (Colour online) Decomposition of the Band-3 spin textures calculated with DFT (solid blocks) and with the corresponding tensorial fits (dashed lines) for $\Gamma^{5g}$ (top row) and $\Gamma^{4g}$ (bottom row). Red/Blue indicate positive/negative components (note the $\mathbf{k}/-\mathbf{k}$ symmetry). Panels (a)/(c) and (b)/(d) were calculated, respectively with and without SOC (see text). The outer circles in the plots corresponds to amplitudes for the radial, tangential and axial components of [0.386,0.265,0.022]/[0.267,0.387,0.030] or (0.387,0.301)/(0.301,0.387) for the $\Gamma^{5g}/\Gamma^{4g}$ phase, respectively, with [] or without () SOC respectively.
